# Supplementary material for: Validating Network Protocol Parsers with Traceable RFC Document Interpretation
Source: arXiv:2504.18050 source file (2025-04-25)
Supplement: Supplementary file 1 [file Appendix.tex]

\newpage
\appendix
\section{Bug List}
\Cref{tab:buglist} presents the complete bug list. For each bug, we describe its root cause, classify it as new or pre-existing, and indicate its confirmation status. Based on developers' responses to bug fixes and merges, we assign a severity level to each confirmed bug: Significant (requires immediate attention), Moderate (can be addressed when time permits), or Trivial (no fix necessary).

\begin{table}[h]
\centering
\scriptsize
\caption{Bug List with Severity Categories (Significant: necessitate immediate attention; Moderate: address later when time permits; Trivial: do not require fixing) and Confirm Status.}
\label{tab:buglist}
\begin{tabular}{ccp{7cm}ccc}
\toprule
\textbf{Bug ID} & \textbf{Protocol} & \textbf{Description} & \textbf{New Bug?}& \textbf{Severity} & \textbf{Status} \\
\midrule
1 & BABEL & Miss non-zero check of Interval in ACK\_REQ TLV.&\checkmark & Moderate & PR Approved \\

2 & BABEL & Miss non-zero check of Interval in IHU TLV. &\checkmark& Moderate & PR Approved \\

3 & BABEL & Miss check if the Router-Id is all zeroes or all ones in ROUTER\_ID TLV.&\checkmark & Moderate & PR Approved\\

4 & BABEL & Miss non-zero check of MBZ in PadN TLV.&\checkmark & Moderate & PR Merged \\

5 & BABEL & Miss non-zero check of MBZ in PadN SUBTLV.&\checkmark & Moderate & PR Merged \\

6 & BABEL & Miss non-zero check of Reserved in ACK\_REQ TLV.&\checkmark & Moderate & PR Merged \\

7 & BABEL & Miss non-zero check of Reserved in IHU TLV. &\checkmark& Moderate & PR Merged \\

8 & BABEL & Miss non-zero check of Reserved in ROUTER\_ID TLV.&\checkmark & Moderate & PR Merged \\

9-23 & BABEL & Miss non-zero check for bits 1-15 of Flags. &\checkmark& Moderate & PR Approved \\

24 & BFD & Miss check for flag Multipoint (M) &\checkmark&Significant &  PR Merged \\
25 & BFD & Missing Check for Authentication Section When Flag A is Set. &\checkmark&Significant &  PR Merged\\
26 & BFD & Miss validate packets are long enough for the authentication header. &\checkmark&Significant &  PR Merged\\
27 & BFD & Miss validate packets are long enough for the full authentication section. &\checkmark&Significant &  PR Merged\\
28 & BFD & Miss check invalid Authentication Type. &\checkmark&Significant &  PR Merged\\
29 &BFD & Miss handle Simple Password Authentication. &\checkmark&Significant &  PR Merged\\
30 &BFD & Miss handle Keyed MD5 Authentication. &\checkmark&Significant &  PR Merged\\
31 &BFD & Miss handle Meticulous Keyed MD5 Authentication. &\checkmark&Significant &  PR Merged\\
33 &BFD & Miss handle Keyed SHA1 Authentication. &\checkmark&Significant &  PR Merged\\
33 &BFD & Miss handle Meticulous Keyed SHA1 Authentication. &\checkmark&Significant &  PR Merged\\
34  & IPv4  & Miss IHL constraint checking. &\checkmark & &Reported\\
35  & IPv4  & Miss checking TotalLength with IHL. &\checkmark & &Reported\\      36  & ICMPv4 & Miss version check.&\checkmark & &Reported\\
37 & ICMPv4 & Miss IHL check.&\checkmark & &Reported\\
38  & ICMPv4 & Miss TypeOfService check.&\checkmark & &Reported\\
39  & ICMPv4 & Miss TotalLength check.&\checkmark & &Reported\\
40 & ICMPv4 & Miss Protocol check.&\checkmark & &Reported\\
41 & ICMPv4 & Miss Code check in Destination Unreachable Message.&\checkmark & &Reported\\
42 & ICMPv4 & Miss Code check in Source Quench Message.&\checkmark & &Reported\\
43 & ICMPv4 & Miss Code check in Redirect Message.&\checkmark & &Reported\\
44 & ICMPv4 & Miss Code check in Time Exceeded Message.&\checkmark & &Reported\\
45 & ICMPv4 & Miss Code check in Parameter Problem Message Message.&\checkmark & &Reported\\
46 & ICMPv4 & Miss Code check in Echo Message.&\checkmark & &Reported\\
47 & ICMPv4 & Miss Code check in Echo Reply Message.&\checkmark & &Reported\\
48 & ICMPv4 & Miss Code check in Timestamp Message.&\checkmark & &Reported\\
49 & ICMPv4 & Miss Code check in Timestamp Reply Message.&\checkmark & &Reported\\
50 & ICMPv4 & Miss Code check in Information Request Message.&\checkmark & &Reported\\
51 & ICMPv4 & Miss Code check in Information Reply Message.&\checkmark & &Reported\\
52 & ICMPv6 & Miss Code check in Destination Unreachable Message.&\checkmark & &Reported\\
53 & ICMPv6 & Miss Code check in Packet Too Big Message.&\checkmark & &Reported\\
54 & ICMPv6 & Miss Code check in Time Exceeded Message.&\checkmark & &Reported\\
55 & ICMPv6 & Miss Code check in Parameter Problem Message.&\checkmark & &Reported\\
56 & ICMPv6 & Miss Code check in Echo Message. &\checkmark & &Reported\\
57 & ICMPv6 & Miss Code check in Echo Reply Message. &\checkmark & &Reported\\
58 & ICMPv6 & Miss Unused field check in Destination Unreachable Message. &\checkmark & &Reported\\
59 & ICMPv6 & Miss Unused field check in Time Exceeded Message. &\checkmark & &Reported\\
60 & IPv6 & Miss check version equal to 6. &\checkmark & &Reported\\
61 & IPv6 & TypeError: can't concat str to bytes. &\checkmark & Significant & PR Merged \\
62 & DHCP & Miss OP check.&\checkmark & &Reported\\
63 & DHCP & Miss htype check.&\checkmark & &Reported\\
64 & DHCP & Miss hlen check.&\checkmark & &Reported\\
65 & DHCP & Incorrect unpackOptions. &$\times$ & Significant & PR Merged\\ 
66 & DHCP & Incorrect unpack structure. &\checkmark &Moderate &Confirmed\\ 
67 & TCP  & Miss check DataOffset. &\checkmark & &Reported\\
68 & TCP  & Miss check Reserved. &\checkmark & &Reported\\
69 & TCP  & Miss check truncated packet. &\checkmark & &Reported\\

\bottomrule
\end{tabular}
\end{table}

\section{Case Studies}

\change{We present case studies of two confirmed bugs discovered by \sysname:
} 
\begin{figure}[t]
  \centering

 \includegraphics[clip=true,trim=0mm 0.5mm 0mm 0mm,width=0.9\linewidth]{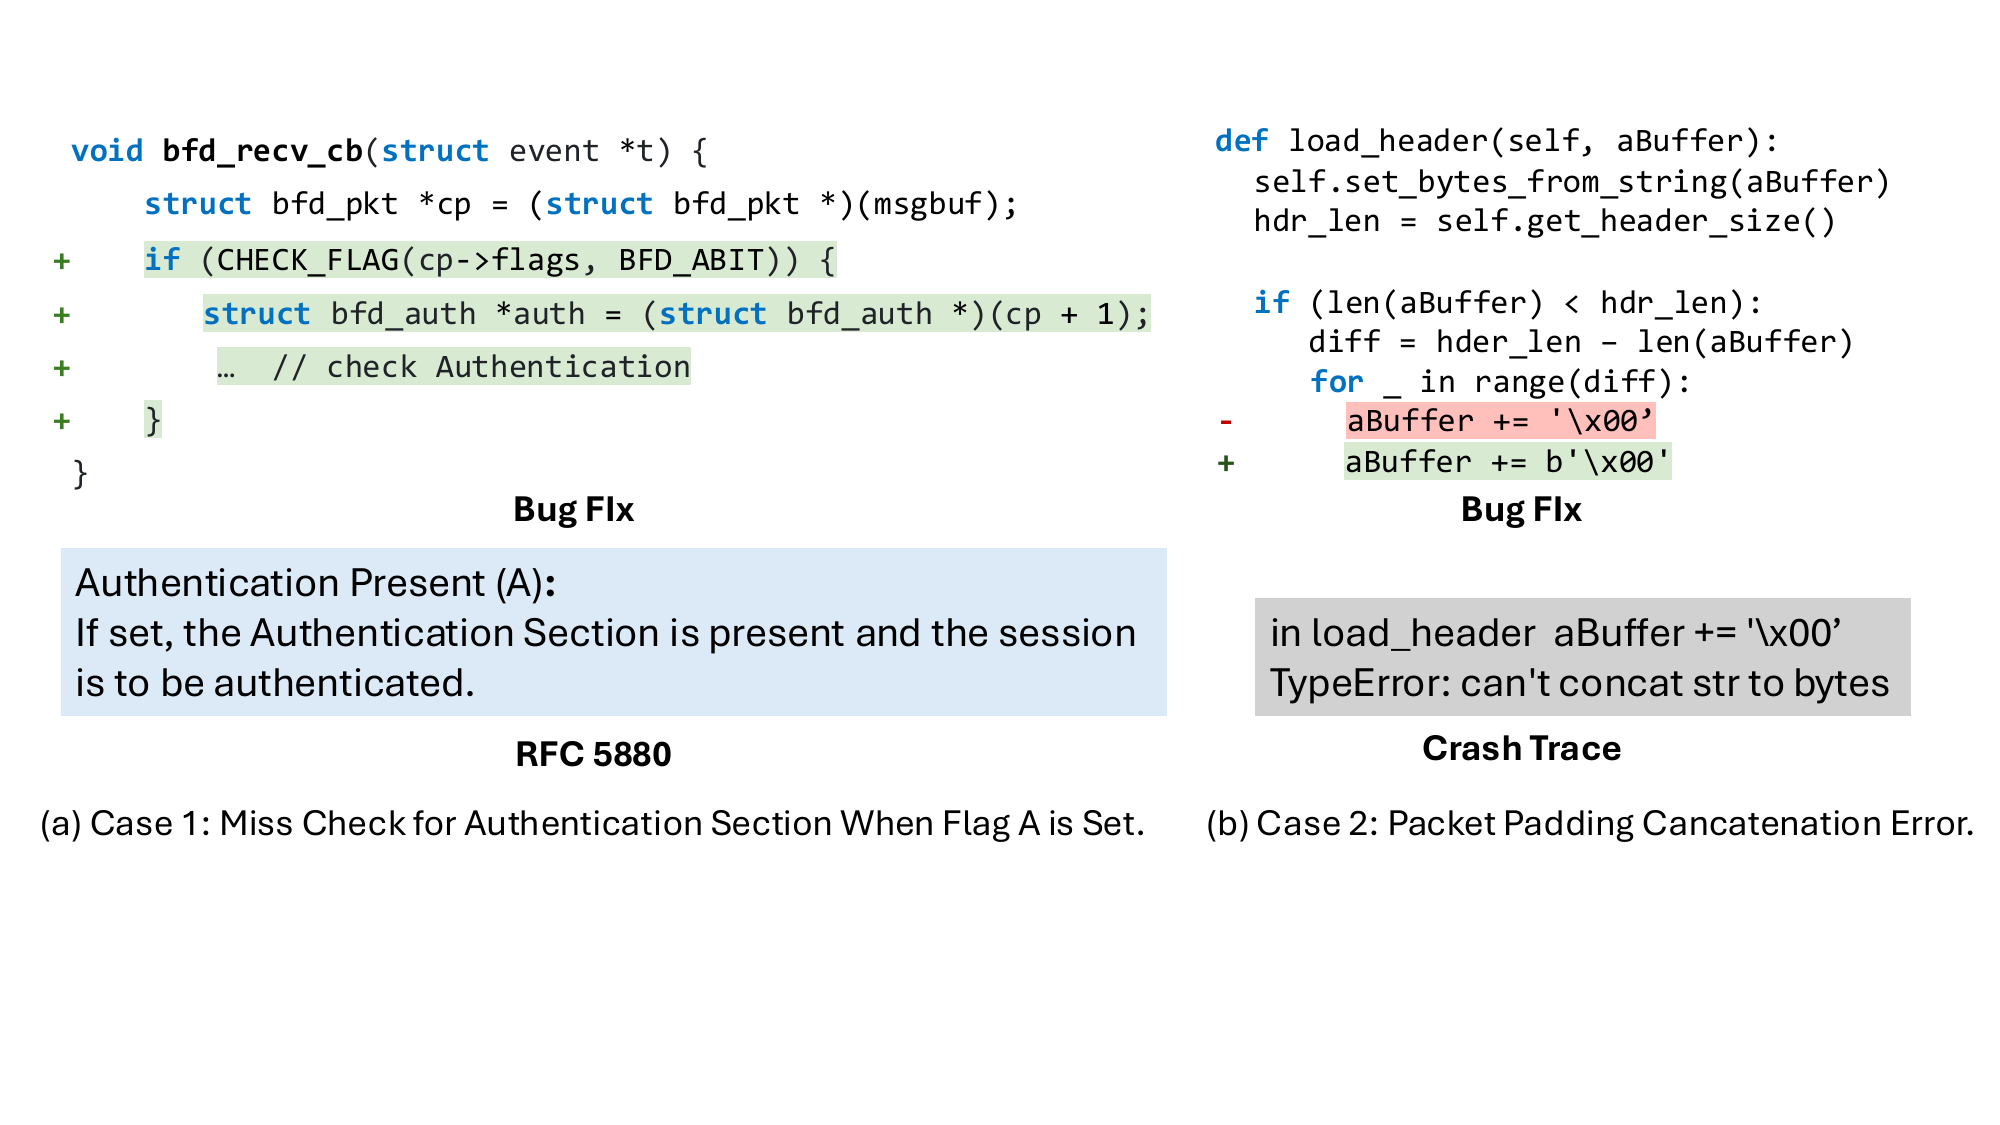}

  \caption{Case Studies.}
  \label{fig:case1}
\end{figure}

\vspace{1mm}
\noindent\change{\textbf{Case 1: Missing Check for Authentication Section When Flag A is Set.}
\Cref{fig:case1} (a) shows a bug fix in the FRRouting BFD implementation and the relevant RFC description.
The original code failed to verify the presence of an Authentication Section when flag A was set.
\sysname detected this issue by generating a malformed packet where flag A was set without an Authentication Section and executing it through the parser, which incorrectly accepted the invalid input.
To resolve this, we created a PR to enforce the check. Our PR was merged by developers immediately.}
\danning{I feel flag A here is not important for understanding the code and it can be a little confusing esp. the "Authentication Present (A):" in blue. Just say it lacks a check here is fine. Is it possible to simplify this case and remove flag A?}

\vspace{1mm}
\noindent
\textbf{Case 2: Packet Padding Concatenation Error.}
\Cref{fig:case1} (b) shows a bug fix for a crash in the Impacket IPv6 implementation, along with the crash trace. The crash occurred when header parsing attempted to zero-pad insufficient data. In Python 3, \texttt{'{\textbackslash}x00'} is treated as a \texttt{string}, causing a TypeError when appended to a bytes buffer: \texttt{aBuffer}.
\sysname triggered this crash by generating an IPv6 packet with insufficient data and running it through the parser. The developers fixed it by adding a \texttt{'b'} prefix to convert \texttt{'{\textbackslash}x00'} to bytes.
